# Supplementary material for: Noise-Induced Barren Plateaus in Variational Quantum Algorithms
Source: arXiv:2007.14384 source file (2024-03-02)

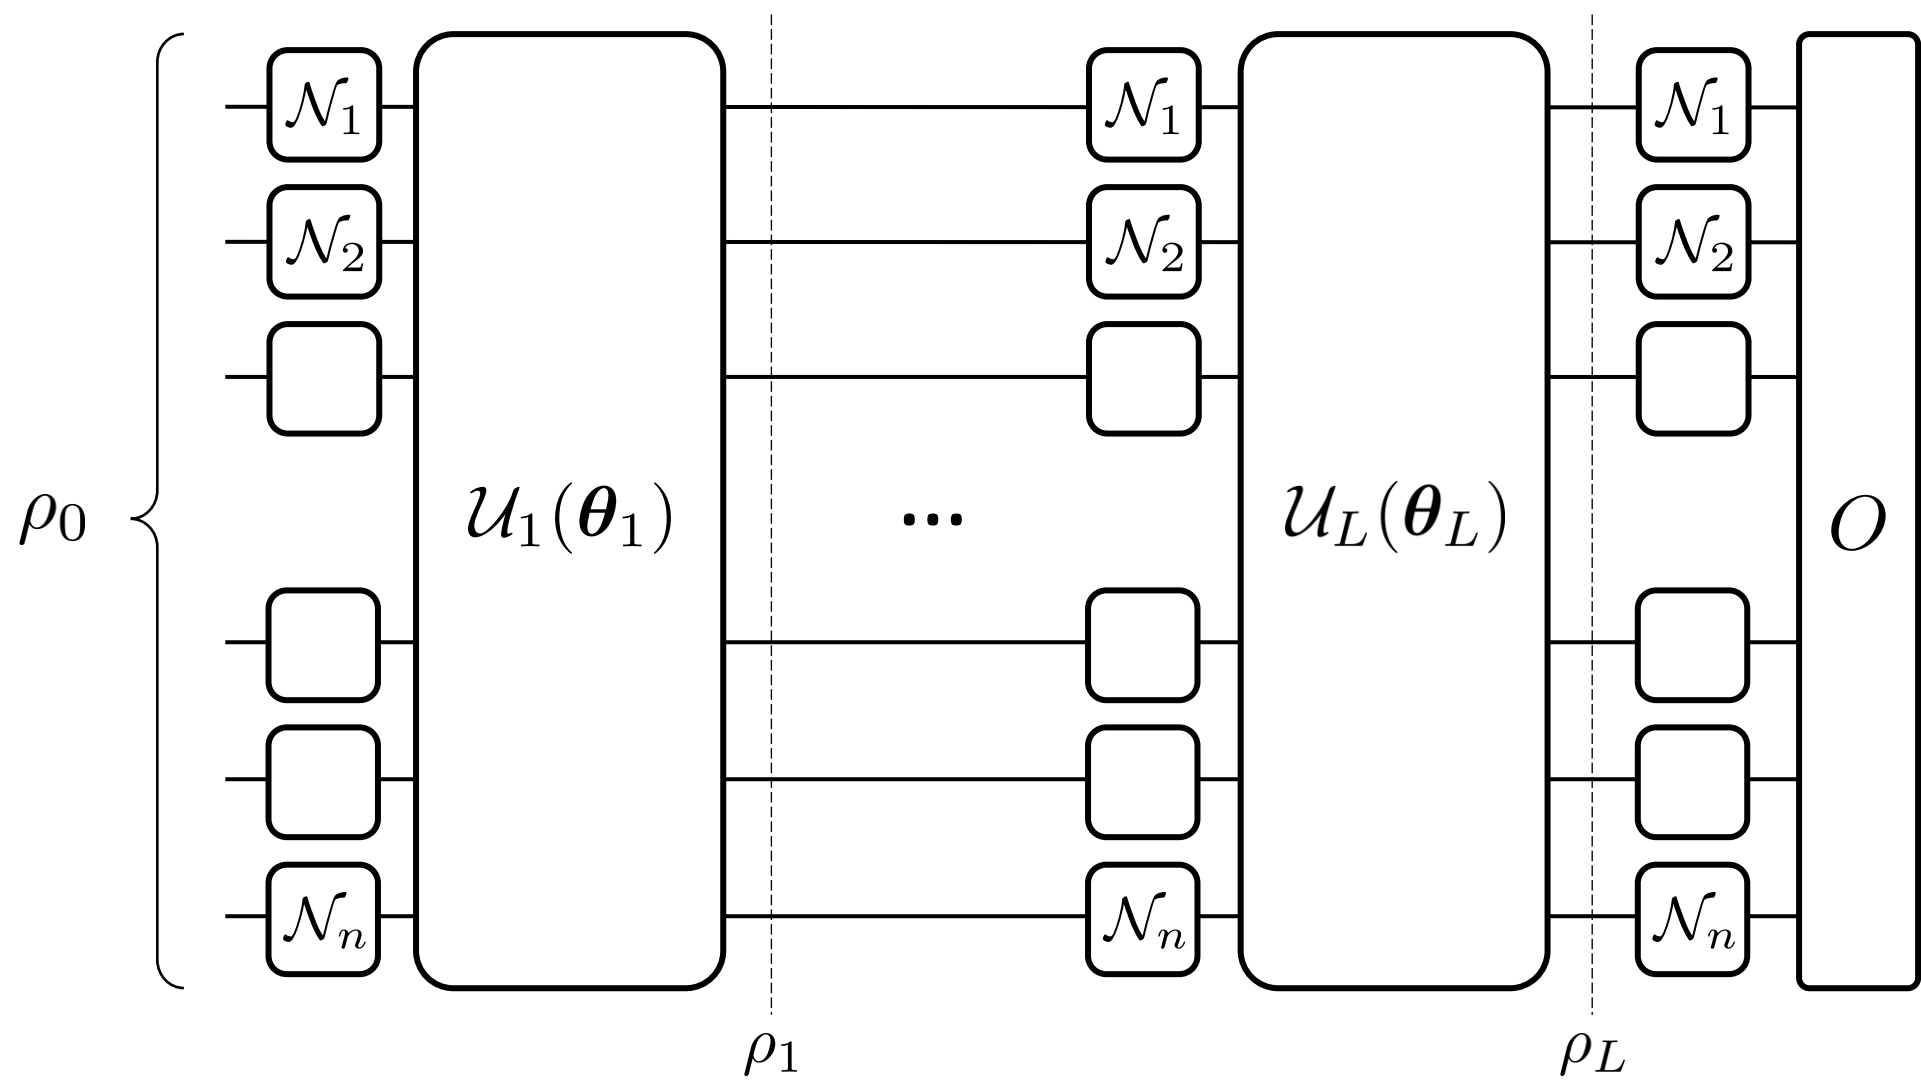

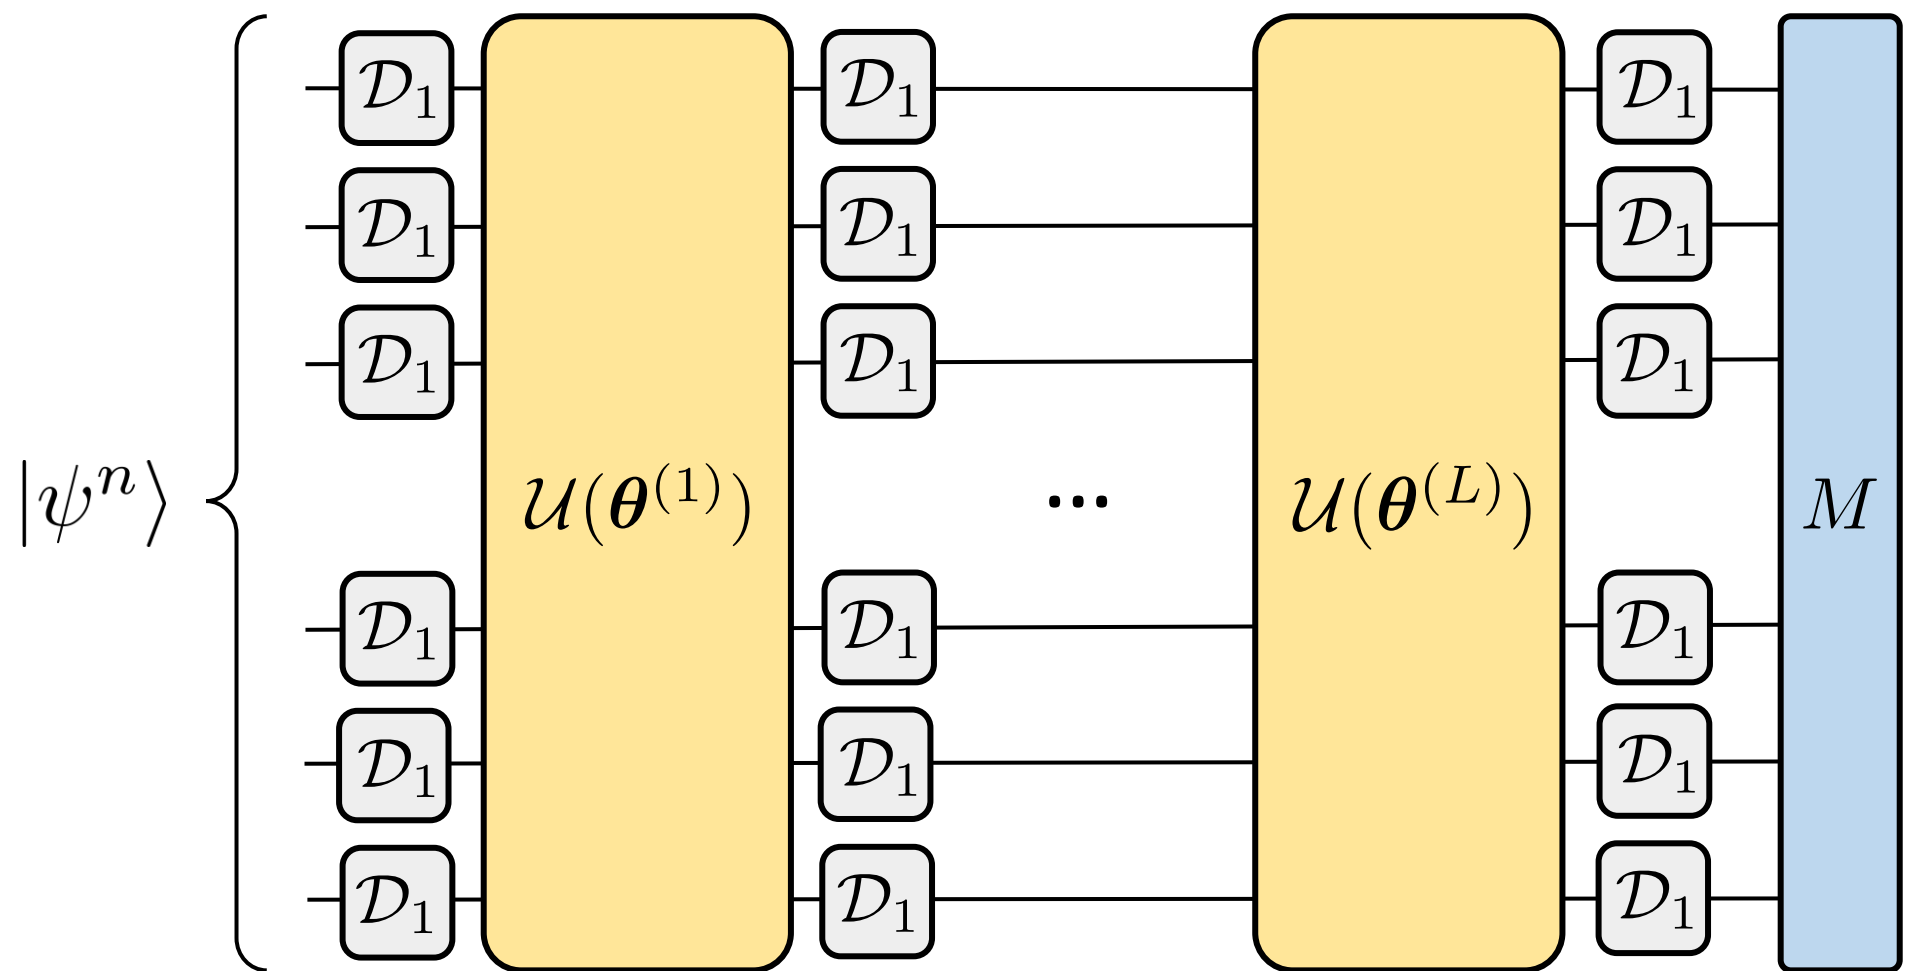

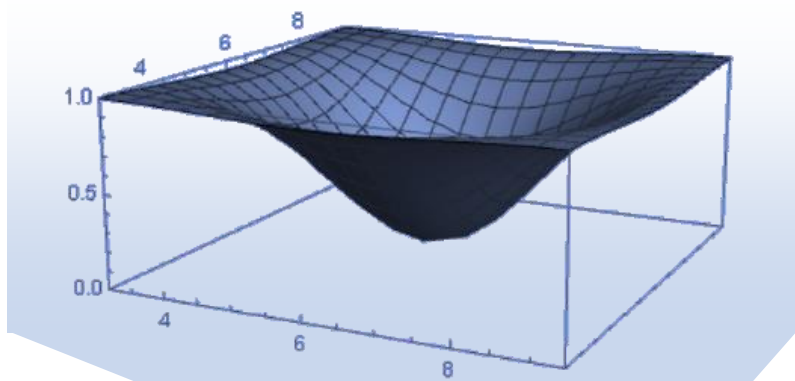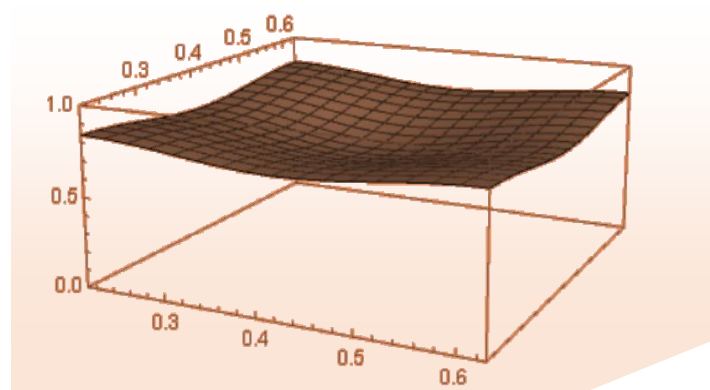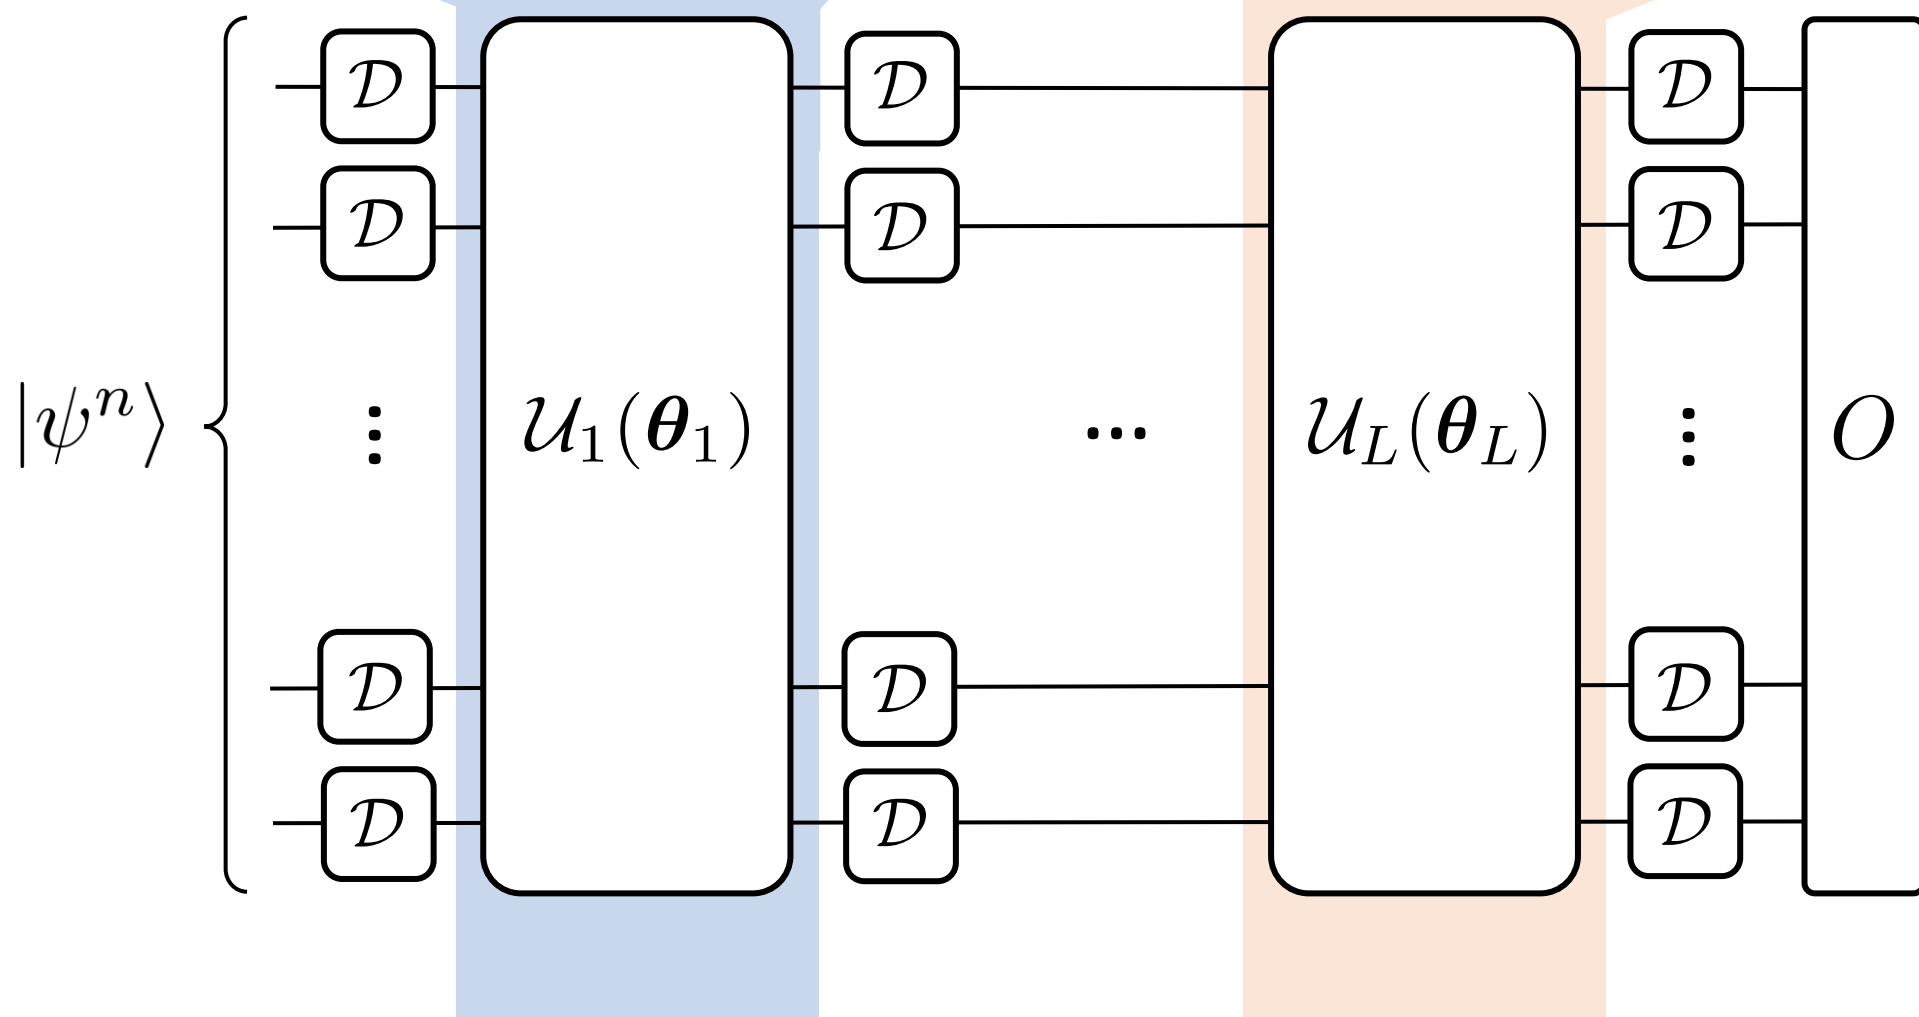

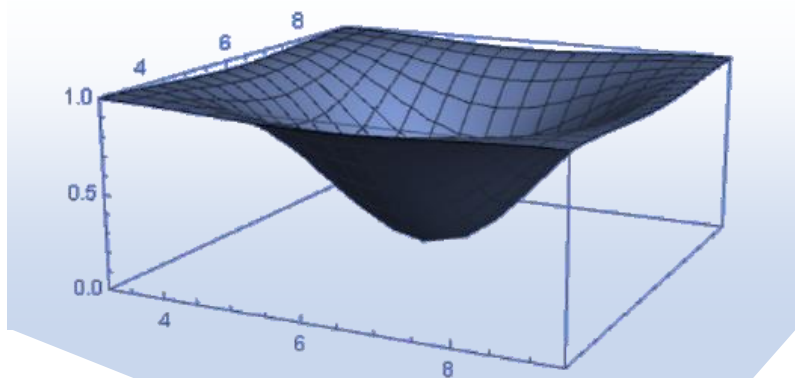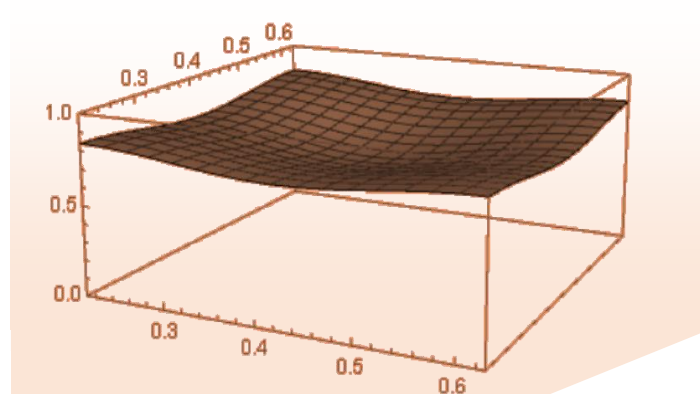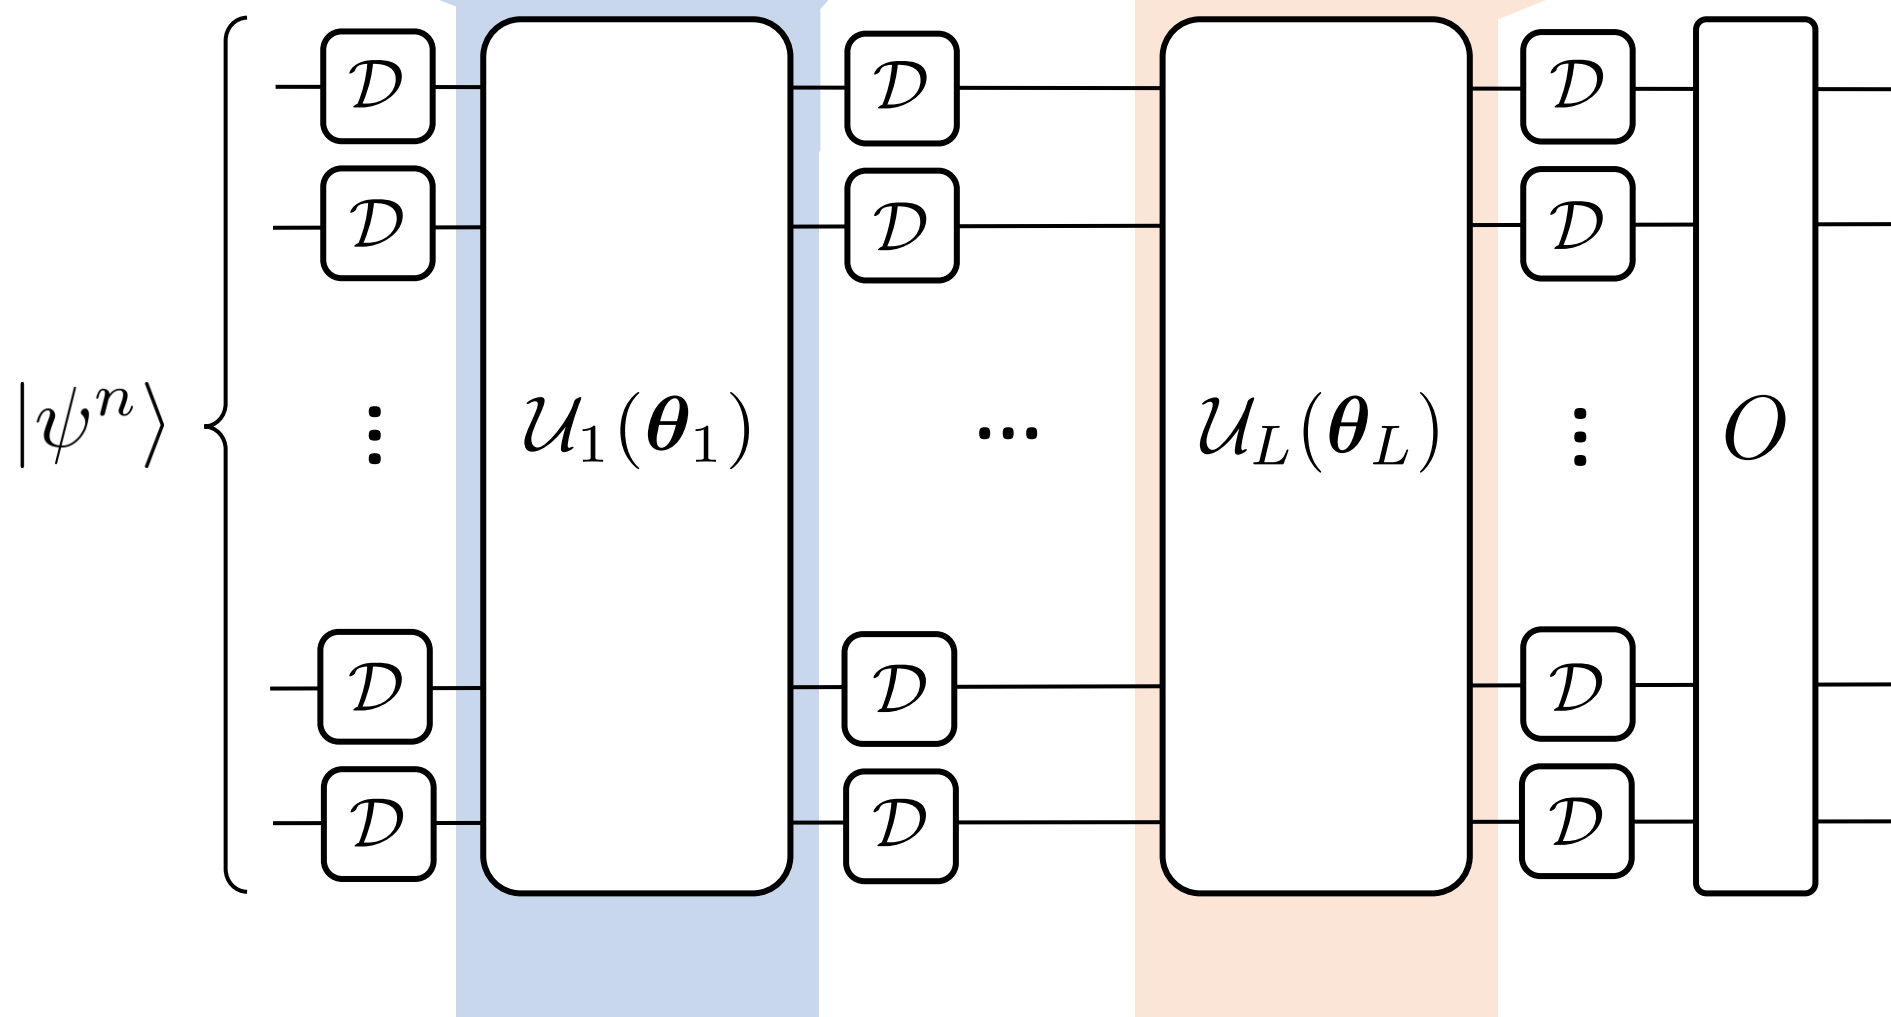



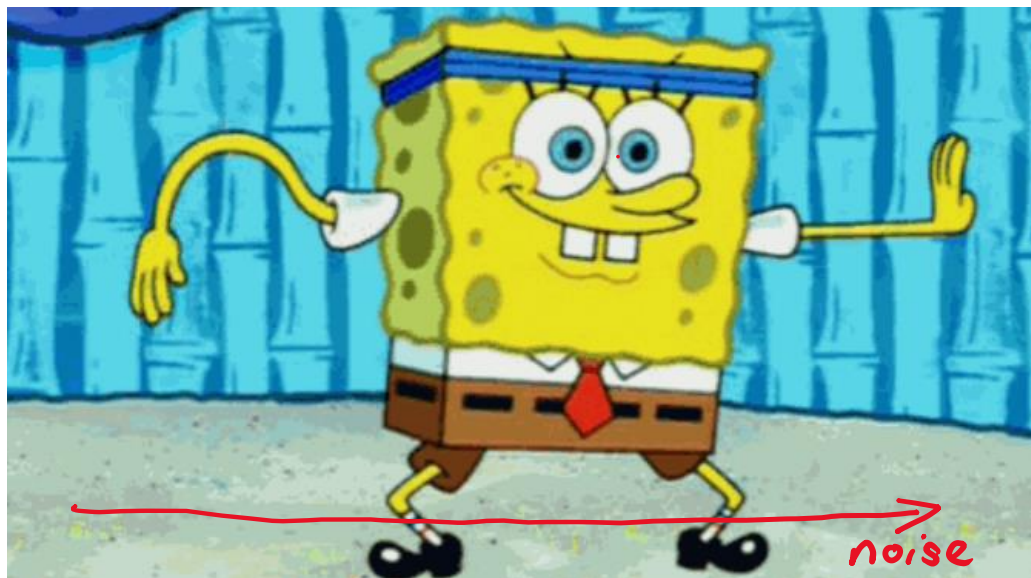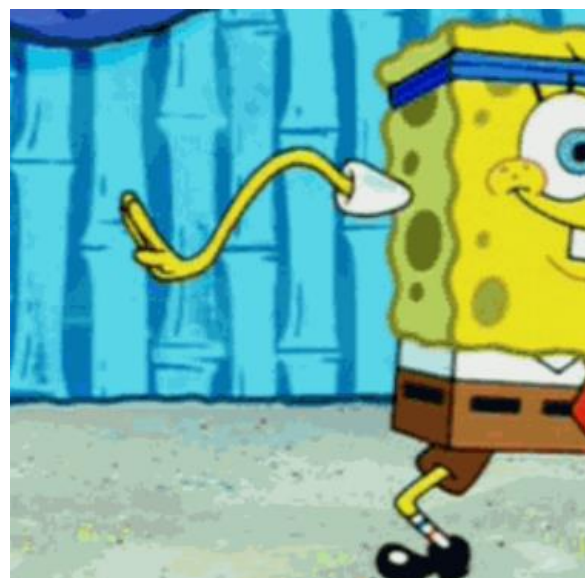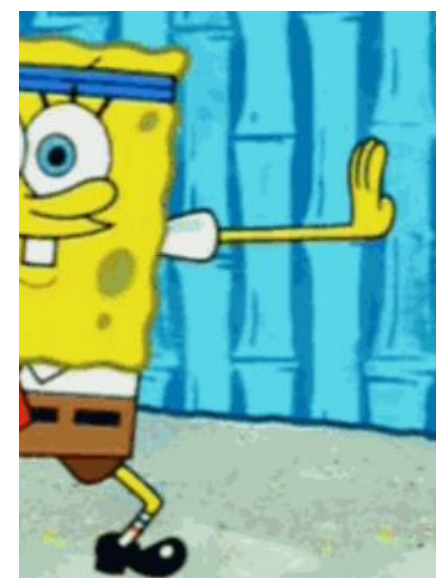

Supplement: Supplementary file 1 [file CircuitSupp.pdf]
